# Supplementary material for: Hypothesis Formalization: Empirical Findings, Software Limitations, and Design Implications
Source: arXiv:2104.02712 source file (2021-04-06)
Supplement: Supplementary file 1 [file appendix.tex]

\begin{appendices}
\section{Appendix}~\label{sec:Appendix}
\subsection{Sampling Published Papers for Published Literature Survey}
As discussed in the Methods section (\autoref{sec:litSurvey}), we started our
analysis of published empirical research papers by open coding six papers from
Psychological Science. 

In case there were any discipline-specific differences, we expanded our sample
to include papers from Psychological Science, Nature, and the Proceedings of
Computer-Human Interaction.  

We randomly sampled publications from each venue. Given each venue's unique
publication frequency, each venue has its own script. All scripts, generated
data used for sampling, and documentation can be found here:~\redacted. 

Since Psychological Science and Nature~\footnote{We looked at papers published
in the journal Nature, not any subsidaries of Nature, such as Nature Astronomy.}
publish multple issues every year, we used a random number generator to select
volume and issue numbers between January 2015 and March 2020 (inclusive). The
list of articles included in each issue was treated as a zero-indexed array. We
also randomly generated wrapping article ``indices'' to pick an article in each issue.
For Nature, we only consider full Research Articles. 

For the Proceedings of Computer-Human Interaction (CHI), we downloaded the
papers from the ACM Digital Library for the years 2016 - 2019.~\footnote{2015
was not included because the ACM Digital Library did not have a folder with all
of the 2015 papers.} Similar to above, we used a script to randomly generate
years and paper numbers to sample the CHI proceedings. 

\textcolor{red}{\section{Plan for proposed changes}}~\label{sec:RevisedAppendix}
\textcolor{red}{See Github repo link~\footnote{\url{https://github.com/emjun/lm_hypothesis}} for most up to date details and code implementing the plan described below.}

\textcolor{red}{In order to randomly sample 1\% of papers from these venues, I will first scrape
a list of paper titles and links (to the papers) for each venue. Then, I will
write a script to randomly select 1\% of the papers from each venue. This script
will output a single CSV of paper titles and links. I will use this output CSV
to manually download the PDFs and any supplemental materials I can find,
including those found on external websites (e.g., Open Science Framework).}

\textcolor{red}{Once I have all the data downloaded, I will process the papers and supplemental
files (usually PDFs) into text files. I will import the text files into
SaturateApp~\footnote{http://www.saturateapp.com/}, a free collaborative
qualitative analysis platform. I will then analyze the written text in the paper
and supplemental materials in Saturate, the code in Saturate (if possible), and
the figures outside of Saturate. I will keep all my notes in Saturate for easy
code development, modification, and summarization.}

\textcolor{red}{I will go through a round of open coding with all the data, a round of code
refinement, and rounds of re-coding. I will then categorize my codes into
hierarchies, which may require further re-coding. Once the codes and code
organization are stable, I will write up my findings. All along the way, I will
take memos to describe what I am finding in the data. }

Original dataset from the Pew Research Center~\cite{Pew:2013}.

From a survey the Pew Research Center conducted in 2013. 
How the dataset for the lab study was created: 
Original data set has 2002 rows/respondents

- Filter for only single adult households --> 485 rows
- Filter for people who completed high school and higher, remove any Don't knows --> 447

- Use State and Community Type - use Zip merge values - Use First major as major
in college - Use "RACE. (1ST MENTION) Which of the following describes your
race? You can select as many as apply. White, Black or African American, Asian
or Asian American or some other race." as race 
- School enrollment? -- combine some values
- Combine was and is college major columns to create College Major

\end{appendices}
