# Supplementary material for: Hypothesis Formalization: Empirical Findings, Software Limitations, and Design Implications
Source: arXiv:2104.02712 source file (2021-04-06)
Supplement: Supplementary file 3 [file tables.tex]

\DeclareUnicodeCharacter{2212}{-}
