# Supplementary material for: Hypothesis Formalization: Empirical Findings, Software Limitations, and Design Implications
Source: arXiv:2104.02712 source file (2021-04-06)
Supplement: Supplementary file 4 [file supp_material.tex]

\section{Working list of supplemental material to submit with paper}
\subsection{Literature Survey}
\begin{enumerate}
    \item Table of papers, summary, contribution types
    \item Reorderable matrices for all
\end{enumerate}

\subsection{Lab Study}
\begin{enumerate}
    \item Pre-study survey
    \item Instructions for all tasks
    \item Post-study survey
\end{enumerate}

\subsection{Tools Analysis}
\begin{enumerate}
    \item Table identifying/aggregating info about the tools
\end{enumerate}
